# Supplementary material for: Inverse probability of treatment weighting with generalized linear outcome models for doubly robust estimation
Source: arXiv:2309.05531 ancillary file (2023-09-11)
Supplement: Supplementary file 1 [file supplement.pdf]

# Supporting Information: "Inverse probability of treatment weighting with generalized linear outcome models for doubly robust estimation"

## S1 Proof of double robustness of Canonical link GLM or linear regression in combination with IPW after regression standardization

Let $X$, $Y$ and $\boldsymbol{Z}$ be the exposure, outcome and a measured confounder, respectively. We assume that $X$ is binary, but make no assumption about $Y$ and $\boldsymbol{Z}$. We will consider the properties of the following estimation procedure. First, the analyst fits a model $p(X=1|\boldsymbol{Z}) = g(\boldsymbol{Z};\boldsymbol{\alpha})$, via some consistent estimator to obtain an estimate $\hat{\boldsymbol{\alpha}}$. Then, the analyst fits a GLM for the outcome via MLE of the form

$$q\{E(Y|X,\boldsymbol{Z})\} = \gamma_0 + \beta X + m(X,\boldsymbol{Z};\boldsymbol{\gamma}),$$

in combination with the weights

$$W(X,\boldsymbol{Z};\hat{\boldsymbol{\alpha}}) = \frac{X}{g(\boldsymbol{Z};\hat{\boldsymbol{\alpha}})} + \frac{1-X}{1-g(\boldsymbol{Z};\hat{\boldsymbol{\alpha}})}.$$

The function $m(X,\boldsymbol{Z};\boldsymbol{\gamma})$ is such that $m(0,0;\boldsymbol{\gamma}) = 0$. It does not need to depend on $X$, but it may, if, for instance, the model contains interactions between $X$ and $\boldsymbol{Z}$. Define $\theta = (\gamma_0, \beta, \boldsymbol{\gamma})$. Thus, we obtain $\theta$ by solving the equation system

$$H(\theta) = \frac{1}{n}\sum_i \left[ W(X_i,\boldsymbol{Z}_i;\hat{\boldsymbol{\alpha}}) \left\{ \begin{array}{c} 1 \\ X_i \\ m'(X_i,\boldsymbol{Z}_i,\boldsymbol{\gamma}) \end{array} \right\} [Y_i - q^{-1}\{\gamma_0 + \beta X_i + m(X_i,\boldsymbol{Z}_i;\boldsymbol{\gamma})\}] \right] = 0 \quad (1)$$

where $m'(X_i,\boldsymbol{Z}_i,\boldsymbol{\gamma}) = \frac{dm(X_i,\boldsymbol{Z}_i,\boldsymbol{\gamma})}{d\boldsymbol{\gamma}}$, for the estimates of $\boldsymbol{\gamma}$ and $\beta$ and $\gamma_0$. All score equations for the MLE fit of a GLM with a canonical link function $q(\cdot)$ will be of the form $H(\theta)$, thus we know that this holds for all canonical link GLM fit via weighted MLE. Additionally, regardless of the outcome type, the OLS estimating equations always take this form with identity link function $q(x) = x$.

If the model for $E(Y|X,\boldsymbol{Z})$ is correctly specified for confounding, then the equations for $(\gamma_0, \beta, \boldsymbol{\gamma})$ are unbiased at the true value of these parameters, regardless of how the weights $W(X,\boldsymbol{Z};\hat{\boldsymbol{\alpha}})$ are specified. We thus conclude: **If the model for $E(Y|X,\boldsymbol{Z})$ is correctly specified for confounding, then the estimator of $(\gamma_0, \beta, \boldsymbol{\gamma})$ is consistent for the true parameters, regardless of whether or not $g(\boldsymbol{Z};\hat{\boldsymbol{\alpha}})$ is correctly specified. Then the plug-in standardization estimator**

$$\hat{E}\{\hat{E}(Y|X=x,\boldsymbol{Z})\} = \sum_{i=1}^{n} q^{-1}\{\hat{\gamma}_0 + \hat{\beta}x + m(x,\boldsymbol{Z}_i;\hat{\boldsymbol{\gamma}})\}/n,$$

**is consistent for $E\{Y(x)\}$.**

Now, consider the case when $g(\boldsymbol{Z};\boldsymbol{\alpha})$ is correctly specified for confounding, but not necessarily the model for $E(Y|X,\boldsymbol{Z})$. Then, taking conditional expectations of the top 2 elements of $H(\theta)$ inside the sum gives

$$E\left[ W(X,\boldsymbol{Z};\boldsymbol{\alpha}) \left\{ \begin{array}{c} 1 \\ X \end{array} \right\} [Y - q^{-1}\{\gamma_0 + \beta X + m(X,\boldsymbol{Z};\boldsymbol{\gamma})\}] \middle| X, Z \right]$$
$$= \frac{1}{p(X|\boldsymbol{Z})} \left\{ \begin{array}{c} 1 \\ X \end{array} \right\} [E(Y|X,\boldsymbol{Z}) - q^{-1}\{\gamma_0 + \beta X + m(X,\boldsymbol{Z};\boldsymbol{\gamma})\}],$$

so that

$$
\begin{aligned}
&E\left[W(X,\boldsymbol{Z};\boldsymbol{\alpha})\begin{pmatrix}1\\X\end{pmatrix}[Y-q^{-1}\{\gamma_0+\beta X+m(X,\boldsymbol{Z};\boldsymbol{\gamma})\}]\middle|\boldsymbol{Z}\right]\\
&=\begin{pmatrix}1\\0\end{pmatrix}[E(Y|X=0,\boldsymbol{Z})-q^{-1}\{\gamma_0+\beta\times 0+m(0,\boldsymbol{Z};\boldsymbol{\gamma})\}]\\
&+\begin{pmatrix}1\\1\end{pmatrix}[E(Y|X=1,\boldsymbol{Z})-q^{-1}\{\gamma_0+\beta\times 1+m(1,\boldsymbol{Z};\boldsymbol{\gamma})\}]
\end{aligned}
$$

and

$$
\begin{aligned}
&E\left[W(X,\boldsymbol{Z};\boldsymbol{\alpha})\begin{Bmatrix}1\\X\end{Bmatrix}[Y-q^{-1}\{\gamma_0+\beta X+m(X,\boldsymbol{Z};\boldsymbol{\gamma})\}]\right]\\
&=\begin{pmatrix}1\\0\end{pmatrix}(E\{E(Y|X=0,\boldsymbol{Z})\}-E[q^{-1}\{\gamma_0+\beta\times 0+m(0,\boldsymbol{Z};\boldsymbol{\gamma})\}])\\
&+\begin{pmatrix}1\\1\end{pmatrix}(E\{E(Y|X=1,\boldsymbol{Z})\}-E[q^{-1}\{\gamma_0+\beta\times 1+m(1,\boldsymbol{Z};\boldsymbol{\gamma})\}]).
\end{aligned}
$$

Setting these expressions to 0 gives that the estimate of $(\gamma_0,\beta,\boldsymbol{\gamma})$ asymptotically satisfies the relations

$$
\begin{aligned}
E\{E(Y|X=0,\boldsymbol{Z})\}-E[q^{-1}\{\gamma_0+\beta\times 0+m(0,\boldsymbol{Z};\boldsymbol{\gamma})\}]=0\\
E\{E(Y|X=1,\boldsymbol{Z})\}-E[q^{-1}\{\gamma_0+\beta\times 1+m(1,\boldsymbol{Z};\boldsymbol{\gamma})\}]=0.
\end{aligned}
\tag{2}
$$

The 'plug-in' estimator of $E\{E(Y|X=x,\boldsymbol{Z})\}$ is

$$\sum_{i=1}^{n} q^{-1}\{\hat{\gamma}_0+\hat{\beta}x+m(x,\boldsymbol{Z}_i;\hat{\boldsymbol{\gamma}})\}/n,$$

and converges in probability to $E[q^{-1}\{\gamma_0+\beta x+m(1,\boldsymbol{Z};\boldsymbol{\gamma})\}]$ as $n$ goes infinity even if the model $q^{-1}\{\gamma_0+\beta x+m(1,\boldsymbol{Z};\boldsymbol{\gamma})$ is misspecified.

Thus, we conclude: **If the model for $p(X=1|\boldsymbol{Z})$ is correctly specified for confounding, then the plug-in estimator of the standardized mean is consistent for $E\{Y(x)\}$, regardless of whether or not the model for $E(Y|X,\boldsymbol{Z})$ is correctly specified.**

■

This has an important implication. Suppose that the true mean $E(Y|X,\boldsymbol{Z})$ is given by

$$q\{E(Y|X,\boldsymbol{Z})\}=\gamma_0+\beta X+m(\boldsymbol{Z};\boldsymbol{\gamma}),\tag{3}$$

where the true function $m(\boldsymbol{Z};\boldsymbol{\gamma})$ does not depend on $X$, and is not necessarily equal to the assumed function $m(X,\boldsymbol{Z};\boldsymbol{\gamma})$. Suppose further that $g$ is the identity link or log link. In this case, the plug-in estimate of the standardized mean is identical to the estimate of $\beta$ obtained from $H(\theta)$. We thus conclude **If the model for $p(X=1|\boldsymbol{Z})$ is correctly specified for confounding, and the true mean $E(Y|X,\boldsymbol{Z})$ is given by (3), then the estimator of $\beta$ is consistent for $E\{Y(1)\}-E\{Y(0)\}$, regardless of whether or not the model for $E(Y|X,\boldsymbol{Z})$ is correctly specified.**

Additionally, note that the proof does not rely on the canonical link GLM, simply that the estimating equations are of the form in (1). Provided this is true, it does not matter whether the link is canonical or if the data matches the selected distribution. One can use ordinary least squares or linear regression for any outcome type, and one could use, for example, Poisson with a log link for a binary outcome, and it would retain the doubly robust property.

## S1.1 Efficient Influence Function

One could also consider this by starting with the efficient influence function (EIF) for $E[E\{Y|X=1,\boldsymbol{Z}\}] = \psi_1$, which is

$$\phi(\boldsymbol{O}) = E\{Y|X,\boldsymbol{Z}\} + \frac{X}{P(X=1|\boldsymbol{Z})}[Y - E\{Y|X,\boldsymbol{Z}\}] - \psi_1$$

with $\boldsymbol{O} = (X, Y, \boldsymbol{Z})$. Using generic versions of our parametric models in the main text in place of the unknown quantities we obtain:

$$\phi(\boldsymbol{O}_i) = q^{-1}\{\gamma_0 + \beta + m(1, \boldsymbol{Z}_i; \boldsymbol{\gamma})\} + \frac{X_i}{g(\boldsymbol{Z}_i; \boldsymbol{\alpha})}[Y_i - q^{-1}\{\gamma_0 + \beta + m(1, \boldsymbol{Z}_i; \boldsymbol{\gamma})\}] - \psi_1.$$

This suggests the estimator:

$$\frac{1}{n}\sum_i q^{-1}\{\hat{\gamma}_0 + \hat{\beta} + m(1, \boldsymbol{Z}_i; \hat{\boldsymbol{\gamma}})\} + \frac{X_i}{g(\boldsymbol{Z}_i; \hat{\boldsymbol{\alpha}})}[Y_i - q^{-1}\{\hat{\gamma}_0 + \hat{\beta} + m(1, \boldsymbol{Z}_i; \hat{\boldsymbol{\gamma}})\}]. \tag{4}$$

By equation (2) and the second component of equation (1), we see that the IPTW GLM estimator is of this form.

Rearranging the terms, we have that this estimator also takes the form

$$\frac{1}{n}\sum_i \left[\frac{X_i Y_i}{g(\boldsymbol{Z}_i; \hat{\boldsymbol{\alpha}})} - \frac{X_i - g(\boldsymbol{Z}_i; \hat{\boldsymbol{\alpha}})}{g(\boldsymbol{Z}_i; \hat{\boldsymbol{\alpha}})} q^{-1}\{\hat{\gamma}_0 + \hat{\beta} + m(1, \boldsymbol{Z}_i; \hat{\boldsymbol{\gamma}})\}\right],$$

which is the form of the estimator of [Funk et al., 2011]. Hence both the IPTW GLM and [Funk et al., 2011] estimators set the empirical version of the efficient influence function to zero, albeit with different estimators of $\beta$ and $\boldsymbol{\gamma}$. Thus when either working model is correctly specified for confounding, both estimators are consistent for $E\{Y(1)\}$. Since both estimators solve the empirical efficient influence function, when both the models are correctly specified for confounding, the two forms of the estimators have the same asymptotic distribution, which we show by showing they have the same influence function.

Denote the two working models $g(\boldsymbol{Z};\alpha)$ and $r_1(\boldsymbol{Z};\theta) = q^{-1}\{\gamma_0 + \beta + m(1, \boldsymbol{Z}; \boldsymbol{\gamma})\}$ with $\theta = (\gamma_0, \beta, \boldsymbol{\gamma})$. To make it clear, $r_1(\boldsymbol{Z};\theta)$ is the working model for $E(Y|X=1,\boldsymbol{Z})$. Let $\tau = (\alpha, \theta)$ and let $\tau^*$ denote the limit in probability of the estimator $\hat{\tau}$ obtained for instance, by MLE, or any other estimation procedure that produces a consistent estimator by which we mean that $\hat{\alpha}$ is consistent for $\alpha_0$ in case the working model $g(\boldsymbol{Z};\alpha)$ is correctly specified with $\alpha_0$ denoting the true value of $\alpha$, and likewise with $\hat{\theta}$. In any case $n^{1/2}(\hat{\tau} - \tau^*) = n^{-1/2}\sum_i \phi_{\tau^*}(\boldsymbol{O}_i) + o_P(1)$, ie $\phi_{\tau^*} = \{\phi_{\alpha^*}, \phi_{\theta^*}\}^T$ is the corresponding influence function (see page 31, equation 3.6, in Tsiatis [2006]), and $\boldsymbol{O} = (X, Y, \boldsymbol{Z})$. It follows by a standard Taylor expansion that the influence function of the proposed estimator $\hat{\psi}_1(\hat{\tau})$ is

$$\Phi_{1i} = \phi_1(\boldsymbol{O}_i; \tau^*) + \mathbb{K}_1(\tau^*)\phi_{\alpha^*}(\boldsymbol{O}_i) + \mathbb{L}_1(\tau^*)\phi_{\theta^*}(\boldsymbol{O}_i)$$

where

$$\mathbb{K}_1(\tau^*) = -E\left[X\frac{\dot{g}(\boldsymbol{Z}, \boldsymbol{\alpha^*})}{[g(\boldsymbol{Z}, \boldsymbol{\alpha^*})]^2}\{Y - r_1(\boldsymbol{Z};\theta^*)\}\right],$$

and

$$\mathbb{L}_1(\tau^*) = E\left\{\frac{\dot{r}_1\{Z;\theta^*\}}{g(\boldsymbol{Z}, \boldsymbol{\alpha^*})}(g(\boldsymbol{Z}, \boldsymbol{\alpha^*}) - X)\right\}$$

with $\dot{g}(\boldsymbol{Z}, \boldsymbol{\alpha^*}) = \frac{\partial g(\boldsymbol{Z}, \boldsymbol{\alpha})}{\partial \boldsymbol{\alpha}}$ evaluated at $\alpha^*$, and likewise with $\dot{r}_1$. Note that $\mathbb{K}_1(\tau^*) = 0$ and $\mathbb{L}_1(\tau^*) = 0$ when the two working models are correctly specified for confounding, in which case the asymptotic distribution of the estimators follows from that of the efficient influence function alone.

Hence, these estimators are asymptotically equivalent when both working models are correctly specified for confounding and should be nearly equivalent in most cases, even in finite samples, although the difference may occur if one fits two outcome models, one for each level of $X$, as suggested in Funk et al. [2011]. The fitting of the models, even if only one outcome model is used, may also cause minor numeric differences due to the fitting of the outcome model unweighted versus weighted likelihood.

Additionally, when both working models are correctly specified for confounding, both estimators are efficient as they align with an estimator suggested by the efficient influence function, and their variance is given by 1 over $n$ times the variance of the efficient influence function, thus reaching the semiparametric lower bound for efficiency. We expand on the variance and an estimator of it in the next section.

# S2 Influence function based standard error estimator

We here describe an influence function based standard error estimator. We require that at least one of the working models is correctly specified for confounding but not necessarily both, which is required for consistent estimation of the ACE. Our estimator for the standard error for our estimator of $\psi_1 = E\{Y(1)\}$ has three parts as described in the following. As above, the two working models are denoted $g(\boldsymbol{Z};\alpha)$ and $r_1(\boldsymbol{Z};\theta) = q^{-1}\{\gamma_0 + \beta + m(1, \boldsymbol{Z}; \boldsymbol{\gamma})\}$ with $\theta = (\gamma_0, \beta, \boldsymbol{\gamma})$. To make it clear, $r_1(\boldsymbol{Z};\theta)$ is the working model for $E(Y|X = 1, \boldsymbol{Z})$. Let $\tau = (\alpha, \theta)$ and let $\tau^*$ denote the limit in probability of the estimator $\hat{\tau}$ obtained, for instance, by MLE, or any other estimation procedure that produces a consistent estimator by which we mean that $\hat{\alpha}$ is consistent for $\alpha_0$ in case the working model $g(Z;\alpha)$ is correctly specified for confounding with $\alpha_0$ denoting the true value of $\alpha$, and likewise with $\hat{\theta}$. Thus, $n^{1/2}(\hat{\tau} - \tau^*) = n^{-1/2}\sum_i \phi_{\tau^*}(O_i) + o_P(1)$, ie $\phi_{\tau^*} = \{\phi_{\alpha^*}, \phi_{\theta^*}\}^T$ is the corresponding influence function (see page 31, equation 3.6, in Tsiatis [2006]), and $O = (X, Y, Z)$. It follows by a standard Taylor expansion that the influence function of the proposed estimator $\hat{\psi}_1(\hat{\tau})$ is

$$\Phi_{1i} = \phi_1(O_i; \tau^*) + \mathbb{K}_1(\tau^*)\phi_{\alpha^*}(O_i) + \mathbb{L}_1(\tau^*)\phi_{\theta^*}(O_i)$$

where

$$\mathbb{K}_1(\tau^*) = -E\left[X\frac{\dot{g}(\boldsymbol{Z}, \boldsymbol{\alpha^*})}{[g(\boldsymbol{Z}, \boldsymbol{\alpha^*})]^2}\{Y - r_1(\boldsymbol{Z}; \theta^*)\}\right],$$

and

$$\mathbb{L}_1(\tau^*) = E\left\{\frac{\dot{r}_1\{Z;\theta^*\}}{g(\boldsymbol{Z}, \boldsymbol{\alpha^*})}(g(\boldsymbol{Z}, \boldsymbol{\alpha^*}) - X)\right\}$$

with $\dot{g}(\boldsymbol{Z}, \boldsymbol{\alpha^*}) = \frac{\partial g(\boldsymbol{Z}, \boldsymbol{\alpha})}{\partial \boldsymbol{\alpha}}$ evaluated at $\alpha^*$, and likewise with $\dot{r}_1$. Note that either $\mathbb{K}_1(\tau^*) = 0$ or $\mathbb{L}_1(\tau^*) = 0$ depending on which of the two working models are correctly specified for confounding. The proposed standard error estimator is then $\left\{n^{-2}\sum_i \Phi_{1i}^2\right\}^{1/2}$. Similarly, we can calculate the influence function of $\hat{\psi}_0(\hat{\tau})$ which we denote by $\Phi_0$. Finally, the standard error estimator of our estimator of $E\{Y(1)\} - E\{Y(0)\}$ is given by $\left\{n^{-2}\sum_i(\Phi_{1i} - \Phi_{0,i})^2\right\}^{1/2}$, and this is the SE estimator we use in the main text.

An R function that computes this standard error is as follows. The arguments are the outcome model fit, the propensity model fit, the name of the exposure variable, and the name of the outcome variable.

```
infunc_confint <- function(ofit, wfit, exposurename, outcomename) {


  data <- ofit$data
  data1 <- data0 <- data
  data1[[exposurename]] <- 1
  data0[[exposurename]] <- 0

  n <- nrow(data1)

  est1f <- mean(predict(ofit, newdata = data1, type = "response"))
  est0f <- mean(predict(ofit, newdata = data0, type = "response"))

  # refit using unweighted estimating equations
  ofitunwt <- glm(ofit$formula, family = ofit$family,
                  data = data)

  phat <- predict(wfit, type = "response")


  est1 <- predict(ofitunwt, newdata = data1, type = "response")
  est0 <- predict(ofitunwt, newdata = data0, type = "response")

  XXw <- model.matrix(wfit)
  XXo <- XXo1 <- XXo0 <- model.matrix(ofitunwt)
  XXo1[,exposurename] <- 1
  XXo0[,exposurename] <- 0

  ifweight <- t(vcov(wfit) %*% t(sandwich::estfun(wfit)))
  ifout <- t(vcov(ofit) %*% t(sandwich::estfun(ofitunwt)))


  eifterms1 <- (data[[exposurename]] / phat * (data[[outcomename]] - est1) +
     (est1 - est1f)) / n
  eifterms0 <- ((1 - data[[exposurename]]) / (1 - phat) * (data[[outcomename]] - est0) +
     (est0 - est0f)) / n


  hdot <- family(wfit)$mu.eta(predict(wfit, type = "link"))

  gdot0 <- family(ofit)$mu.eta(predict(ofitunwt, newdata = data0, type = "link"))
  gdot1 <- family(ofit)$mu.eta(predict(ofitunwt, newdata = data1, type = "link"))

  Kterm1 <- (-1/n) * matrix(((data[[exposurename]] * hdot) / phat^2) *
                            (data[[outcomename]] - est1), nrow = 1, ncol = n) %*% XXw
  Kterm0 <- (1/n) * matrix((((1 - data[[exposurename]]) * hdot) / (1 - phat)^2) *
                           (data[[outcomename]] - est0), nrow = 1, ncol = n) %*% XXw

  Lterm1 <- (1/ n) * matrix(gdot1 * (1 - data[[exposurename]]/phat),
    nrow = 1, ncol = n) %*%  XXo1
```

```
  Lterm0 <- (1/ n) * matrix(gdot0 * ((1 - data[[exposurename]])/(1 - phat) - 1),
    nrow = 1, ncol = n) %*%  XXo0

  fullif1 <- cbind(eifterms1, (ifweight %*% t(Kterm1)), (ifout %*% t(Lterm1)))
  fullif0 <- cbind(eifterms0, (ifweight %*% t(Kterm0)), (ifout %*% t(Lterm0)))


  estse <- sqrt(sum((rowSums(fullif1) - rowSums(fullif0))^2))
  est <- est1f - est0f

  c(lower = est - 1.96 * estse, upper = est + 1.96 * estse)


}
```

Table S1 shows the results of a simulation study to assess the bias of the standard error estimators in relation to the empirical standard error over simulated replicates. The estimator based on the influence function that accounts for the estimation of the propensity score and outcome models is accurate in all cases, even when both models are wrong, while the estimator based only on the efficient influence function tends to be too high in these data generation settings.

Table S1: Comparison of the standard error and its estimators. The column labeled emp.se shows the empirical standard deviation of the ACE estimators over 2000 simulated replicates, eif.se shows the average of the standard error estimates based on only the efficient influence function, and infl.se shows the average of the standard error estimates that account for estimation of the propensity score and outcome models.

| setting | type | emp.se | eif.se | infl.se |
|---|---|---|---|---|
| linear | wrong outcome right weights | 0.067 | 0.110 | 0.064 |
| linear | right outcome wrong weights | 0.047 | 0.045 | 0.045 |
| linear | wrong both | 0.084 | 0.085 | 0.084 |
| linear | right both | 0.049 | 0.049 | 0.049 |
| log_poisson | wrong outcome right weights | 0.163 | 0.209 | 0.164 |
| log_poisson | right outcome wrong weights | 0.157 | 0.161 | 0.158 |
| log_poisson | wrong both | 0.211 | 0.212 | 0.211 |
| log_poisson | right both | 0.159 | 0.161 | 0.161 |
| logit_binomial | wrong outcome right weights | 0.013 | 0.019 | 0.014 |
| logit_binomial | right outcome wrong weights | 0.012 | 0.012 | 0.013 |
| logit_binomial | wrong both | 0.018 | 0.018 | 0.018 |
| logit_binomial | right both | 0.012 | 0.012 | 0.012 |
| inverse_gaussian | wrong outcome right weights | 0.001 | 0.001 | 0.001 |
| inverse_gaussian | right outcome wrong weights | 0.001 | 0.001 | 0.001 |
| inverse_gaussian | wrong both | 0.001 | 0.001 | 0.001 |
| inverse_gaussian | right both | 0.001 | 0.001 | 0.001 |

## S3 Canonical Link GLM and score equations

Consider a general exponential family with a log likelihood given by

$$l(\beta) = \sum_i \{y_i\theta_i - c(\theta_i)\}/\phi$$

where the parameterization is given by here $\theta_i = \theta(\mu_i) = \theta(q^{-1}(x_i\beta))$ where $\theta(\mu_i) = c'^{-1}(\mu_i)$ and $\mu_i = E[Y|x_i]$, and $q^{-1}(\cdot)$ is some known and inverse link function. If $q(\mu) = \theta(\mu)$ then $q(\cdot)$ is the canonical link

function and $\theta_i = x_i\beta$. Therefore,

$$l(\beta) = \sum_i \{y_i x_i \beta - c(x_i\beta)\}/\phi$$

and thus the score equations for a fixed $\phi = 1$ is

$$X^T\{y - q^{-1}(X\beta)\} = 0$$

which is exactly the form of estimating equations in 1. Thus a canonical link GLM will always fulfill the requirements of the proof above.

When $q(\mu) \neq \theta(\mu)$ the score equations will have two additional pieces. Then the score equations are given by:

$$Q^T D(\beta)\{y - q^{-1}(X\beta)\} = 0$$

where $Q$ is a matrix with elements

$$Q(\beta)_{ij} = \frac{\partial X_i \boldsymbol{\beta}}{\partial \beta_j}$$

and $D(\boldsymbol{\beta})$ is a diagonal matrix with elements on the diagonal given by $D_{ii} = 1/v\{\mu_i(\boldsymbol{\beta})\}$ where $v(\cdot)$ is the variance function and $v\{\mu_i(\boldsymbol{\beta})\} = c''\{c'^{-1}(q^{-1}(X_i\beta)\}$.

# S4 Code for Real Data Example

```
data <- AF::clslowbwt
head(data)
```

```
  id birth  smoke     race age lwt  bwt    low lbw smoker
1  1     1 1. Yes 3. Other  28 120 2865  0. No   0      1
2  1     2 1. Yes 3. Other  33 141 2609  0. No   0      1
3  2     1  0. No 1. White  29 130 2613  0. No   0      0
4  2     2  0. No 1. White  34 151 3125  0. No   0      0
5  2     3  0. No 1. White  37 144 2481 1. Yes   1      0
6  3     1 1. Yes 2. Black  31 187 1841 1. Yes   1      1
```

```
## propensity score fit

pwfit <- glm(smoker ~ race * age * lwt + I(age^2) + I(lwt^2), data = data,
             family = "binomial")
phat <- predict(pwfit, type = "response")

data$weight <- data$smoker / phat + (1 - data$smoker) / (1 - phat)
## outcome model

outfit <- glm(bwt ~ smoker * (race + age + lwt) + I(age^2) + I(lwt^2),
              data = data, family = "gaussian", weights = weight)

## dummy data, where we set X to 0 and 1

data0 <- data1 <- data
data0$smoker <- 0
data1$smoker <- 1

## predicted counterfactuals
Yhat0 <- predict(outfit, newdata = data0, type = "response")
Yhat1 <- predict(outfit, newdata = data1, type = "response")
```

```r
ATEmean <- mean(Yhat1) - mean(Yhat0)
ATEmean
```

```
[1] -223.6736
```

```r
infunc_confint(outfit, pwfit, "smoker", "bwt")
```

```
      lower       upper
-446.081852   -1.265258
```

```r
## Funk et al. approach

## separate outcome models, unweighted

ofit1 <- glm(bwt ~ (race + age + lwt) + I(age^2) + I(lwt^2),
              data = subset(data, smoker == 1), family = "gaussian")

ofit0 <- glm(bwt ~ (race + age + lwt) + I(age^2) + I(lwt^2),
              data = subset(data, smoker == 0), family = "gaussian")


dr1 <- data$bwt * (data$smoker == 1) / phat -
  predict(ofit1, newdata = data1, type = "response") *
  ((data$smoker == 1) - phat) / phat
dr0 <- data$bwt * (data$smoker == 0) / (1 - phat) +
  predict(ofit0, newdata = data0, type = "response") *
  ((data$smoker == 1) - phat) / (1 - phat)

ATEfunk <- mean(dr1) - mean(dr0)
ATEfunk
```

```
[1] -225.5489
```

```r
## outcome model

outfit <- glm(lbw ~ smoker * (race + age + lwt) + I(age^2) + I(lwt^2),
              data = data, family = "binomial", weights = weight)
```

# References


Michele Jonsson Funk, Daniel Westreich, Chris Wiesen, Til Stürmer, M Alan Brookhart, and Marie Davidian. Doubly robust estimation of causal effects. *American journal of epidemiology*, 173(7):761–767, 2011.

Anastasios A Tsiatis. Semiparametric theory and missing data. 2006.
